# Supplementary material for: Symmetry fractionalization, mixed-anomalies and dualities in quantum spin models with generalized symmetries
Source: arXiv:2307.01266 source file (2025-01-22)
Supplement: Supplementary file 1 [file 2+1d_DW_theory.tex]

Dijkgraaf-witten theories \cite{Dijkgraaf:1989pz} with the gauge group $\mbb Z_n$ are classified by $H^{3}(\mbb Z_n,\ms U(1))\cong \mbb Z_n$. Given an element ${\rm p} \in \mbb Z_{n}$, one may define a topological action as 
\begin{equation}
    S=\frac{i n}{2\pi}\int \widehat{a}\wedge {\rm{d}}a+\frac{i\rm p}{2\pi}\int a\wedge {\rm{d}}a+\frac{i}{2\pi}\int \left[B\wedge a + \widehat{B}\wedge \widehat{a}\right]\,.
    \label{eq:DW_Zn}
\end{equation}
Here we have used a continuum formulation of the Dijkgraaf-Witten (see Sec.~5 of \cite{Kapustin:2014gua}). 
Here $a$ and $\widehat{a}$ are dynamical compact $\ms U(1)$ 1-form gauge fields while $B$ and $\widehat{B}$ are 2-form background gauge fields corresponding to the global 1-form symmetry of the model.
This theory is shown to be equivalent to the more conventional $\mbb Z_n$ gauge formulation in \cite{Dijkgraaf:1989pz} by integrating over $\widehat{a}$.
For simplicity, if we set $B=\widehat{B}=0$, then integrating over $\widehat{a}$ imposes ${\rm{d}}a=0 \ \text{mod} \ 2\pi$ and $\oint a\in \frac{2\pi}{n}\mbb Z$.
Together these two conditions make $a$ a $\mbb Z_n$ gauge field.

Another convenient formulation of the Dijkgraaf-Witten theory is on an oriented simplicial manifold $M$ using the framework of simplicial calculus.
Then instead of $\ms U(1)$ gauge field, we let $\frac{2\pi}{n}a$ and $\frac{2\pi}{n}\widehat{a}$ be 1-cochains $C^{1}(M,\mbb Z_n)$. This mapping is informed by the fact that on-shell the holonomies of these fields are quantized to $\mbb Z_n\subset \ms{U}(1)$.
We choose this normalization such that on each 1-cell, $a$ and $\widehat{a}$ take values in $\left\{0,1,\dots,n\right\}$. Making these substitutions in \eqref{eq:DW_Zn}, one obtaines
\begin{equation}
    S=\frac{2\pi i}{n}\int\left\{\widehat{a}\cup {\rm d}a +{\rm p} a \cup \frac{\rm{d} a}{n} + \left[B\cup a+ \widehat{B}\cup \widehat{a}\right]\right\}\,.
\end{equation}
One can integrate out $\widehat{a}$ such that $a \in Z^{1}(M,\mbb Z_n)$. Upon doing so, it is more rigorous to understand ${\rm d}a/n$ as ${\rm{Bock}}(a)$.
The gauge invariant topological operators in the theory are
\begin{equation}
\begin{split}
    W_{(\rm{q,m})}(\gamma)=\exp\left\{\frac{2\pi i}{n}\oint_{\gamma}\rm{q}a+{\rm}\widehat{a}\right\}\,,
\end{split}
\end{equation}
where ${\rm{q}}\in \rm{Rep}(\mbb Z_n)\cong \mbb Z_n$ and ${\rm{m}}\in \mbb Z_n$.
The correlation functions of the topological line operator can be computed straightforwardly using standard methods \cite{Tiwari:2016zru, Putrov:2016qdo}.
For instance consider two 1-cycles $\gamma_{1}$ and $\gamma_2$ embedded in $M=S^3$ such that they form a Hopf-link. The correlation function of two line operators with support on $\gamma_1$ and $\gamma_2$ is
\begin{equation}
    \Big \langle W_{(\rm{q}_1,\rm{m}_1)}(\gamma_1) W_{(\rm{q}_2,\rm{m}_2)}(\gamma_2) \Big \rangle = \exp\left\{\frac{2\pi i}{n}(\rm{q}_1\rm{m}_2+\rm{q}_2\rm{m}_1)+\frac{4\pi i {\rm p}}{n^2}{\rm m_1m_2}\right\}\,.
\end{equation}
