# Supplementary material for: Symmetry fractionalization, mixed-anomalies and dualities in quantum spin models with generalized symmetries
Source: arXiv:2307.01266 source file (2025-01-22)
Supplement: Supplementary file 2 [file BF_type_Z2_gauge_theory_Hamiltonians.tex]

The toric code and double semion models refer to the fixed point limits of  deconfined phase of the $\mbb Z_{2}$ and twisted $\mbb Z_2$ gauge theory, where the twist is in the sense of Dijkgraaf-Witten theory \cite{Dijkgraaf:1989pz}.
The fixed point Hamiltonians have the form 
\begin{equation}
\begin{split}
    \mathcal H_{\rm{T.C}}&=-\sum_{\ms v}\prod_{\ms e \supset \ms v} \sigma^{z}_{\ms e} - \sum_{\triangle}\prod_{\ms e \subset \partial \triangle}\sigma^{x}_{\ms e}\,, \\
    \mathcal H_{\rm{D.S}}&=-\sum_{\ms v}\prod_{\ms e \supset \ms v} \sigma^{z}_{\ms e}\prod_{\ms e \in \partial {\rm{Hex}}_{\ms v}}i^{\frac{1-\sigma^{x}_{\ms e}}{2}}- \sum_{\triangle}\prod_{\ms e \subset \partial \triangle}\sigma^{x}_{\ms e}\,.
\label{eq:quantum doubles}
\end{split}
\end{equation}
Let us work in the eigen basis of $\sigma^{x}$ such that 
\begin{equation}
    \sigma^{x}_{\ms e}|a\rangle =(-1)^{a[\ms e]}|a\rangle\,, 
\end{equation}
where $a\in C^{1}(\Sigma_{\triangle},\mbb Z_2)$ and $a[\ms e]$ denotes the evaluation of $a$ on the edge $\ms e$. Therefore, we can straightforwardly write the operator in \eqref{eq:quantum doubles} defined on the  faces $\triangle$ as (see Fig.\ref{Fig:sigma_x in gauge basis})
\begin{equation}
    \prod_{\ms e \subset \partial \triangle}\sigma^{x}_{\ms e} = \sum_{a}\exp\left\{i\pi\oint_{\partial \triangle}a\right\}|a\rangle \langle a|
    \equiv
    \exp\left\{i\pi\oint_{\partial \triangle}\widehat{a}\right\}
    \,.
\end{equation}
\begin{figure}[h]
\begin{center}
\includegraphics[width=0.8\textwidth]
{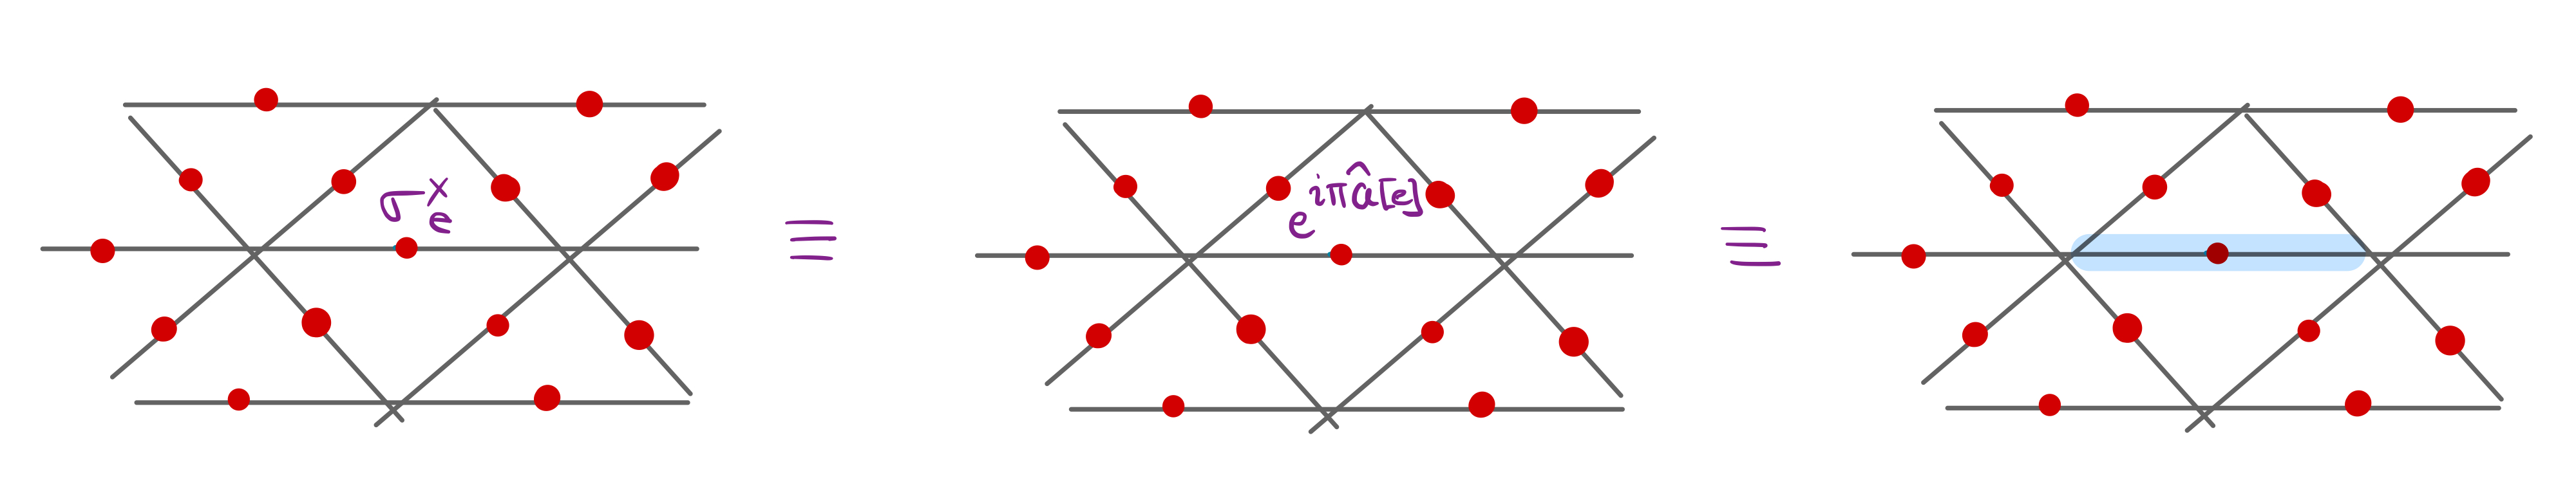}    
\end{center}
\caption{The operator $\sigma^{x}$ in the basis $\left\{|a\rangle\right\}$ is depicted by a blue line on the edge.}
\label{Fig:sigma_x in gauge basis}
\end{figure}

\medskip \noindent Similarly, the operators $\sigma^{z}_{\ms e}$ change the eigenvalue $a[\ms e]$ to $a[\ms e]+ 1 \ \rm{mod} \ 2$. We may describe this operator more generally via a cochain $b\in C^{1}(\Sigma^{\rm{dual}}_{\triangle},\mbb Z_2)$ on the dual lattice $\Sigma^{\rm{dual}}_{\triangle}$. This is possible when $\Sigma$ is two dimensional, since there is a bijection between the edges of the lattice and the dual lattice.
We will denote the dual cochains as green strings on the dual lattice (see Fig.~\ref{Fig:sigma_z in gauge basis})
\begin{figure}[h]
\begin{center}
\includegraphics[width=0.9\textwidth]{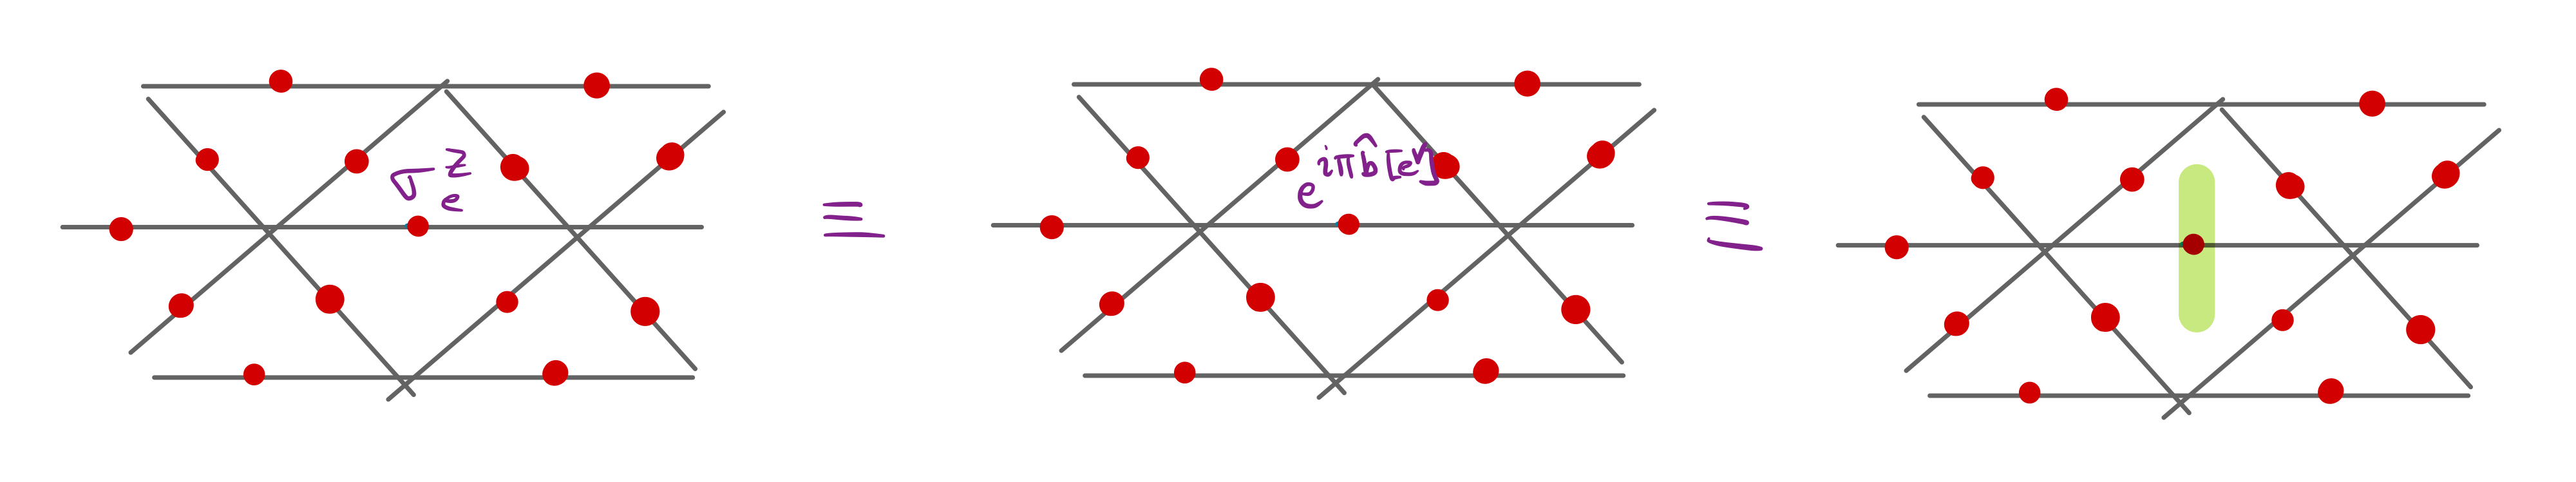}    
\end{center}
\caption{The operator $\sigma^{z}$ in the basis $\left\{|a\rangle\right\}$ is depicted by a green line on an edge $\ms e^{\vee}\subset \Sigma^{\rm{dual}}_{\triangle}$ which is dual to $\ms e \subset \Sigma_{\triangle}$.}
\label{Fig:sigma_z in gauge basis}
\end{figure}

\newl Then the Pauli algebra is represented as the string algebra {\AT{insert a tikz eqn depicting this}}.
With this reinterpretation of the operators acting on the edge Hilbert space, let us reinterpret the Hamiltonian.
It is easy to confirm that there is the following map of operators {\AT{add pictorial depiction of these operators}}
\begin{equation}
\begin{alignedat}{2}
    \prod_{\ms e \subset \partial\triangle} \sigma^{x}_{\ms e} 
    &\longleftrightarrow&& 
    \exp\left\{i\pi \oint_{\partial \triangle} \widehat{a}\right\}\,, \\ 
    \prod_{\ms e \supset \ms v} \sigma^{z}_{\ms e}     &\longleftrightarrow&& 
    \exp\left\{i\pi \oint_{\gamma^{\vee}_{\ms v}}\widehat{b}\right\}\,, \\
    \prod_{\ms e \supset \ms v} \sigma^{z}_{\ms e}\prod_{\ms e \in \partial {\rm{Hex}}_{\ms v}}i^{\frac{1-\sigma^{x}_{\ms e}}{2}}  
    &\longleftrightarrow&& 
    \exp\left\{i\pi \oint_{\gamma^{\vee}_{\ms v}}\widehat{b}+\frac{i\pi}{2}\oint_{\partial \rm{Hex}_{\ms v}}\widehat{\widetilde{a}} \right\}\,,
\end{alignedat}
\end{equation}
where $\gamma^{\vee}_{\ms v}$ is a smallest possible loop on the lattice $\Sigma_{\triangle}^{\rm{dual}}$ linking with the vertex $\ms v \subset \Sigma_{\triangle}$ and $\widehat{\widetilde{a}}$ is the operator corresponding to the $\mbb Z_4 $ lift of $a$.

\newl With this we can re-express the Hamiltonians in \eqref{eq:quantum doubles} as
\begin{equation}
\begin{split}
    \mc H_{\rm{T.C}}&= -  \sum_{\ms v} \exp\left\{i\pi \oint_{\gamma^{\vee}_{\ms v}}\widehat{b}\right\} - \sum_{\triangle}\exp\left\{i\pi \oint_{\partial \triangle} \widehat{a}\right\}\,, \\
   \mc H_{\rm{D.S}}&= -  \sum_{\ms v} \exp\left\{i\pi \oint_{\gamma^{\vee}_{\ms v}}\widehat{b}+\frac{i\pi}{2}\oint_{\partial \rm{Hex}_{\ms v}}\widehat{\widetilde{a}} \right\} - \sum_{\triangle}\exp\left\{i\pi \oint_{\partial \triangle} \widehat{a}\right\}\,,
   \label{eq:TC and DS in loop basis}
\end{split}
\end{equation}
It is useful to define the following line operators
\begin{equation}
    \mc W_{(\ms q, \ms m)}^{(p)}(L) := \exp\left\{
    i\pi \ms q\oint_{\gamma}\widehat{b}+\frac{i\pi p\ms q}{2}\oint_{\gamma^{\vee}}\widetilde{\widehat{a}}
    +i\pi \ms m\oint_{\gamma^{\vee}}\widehat{a}
    \right\}\,. 
    \label{eq:line_operators}
\end{equation}
Here $L=\left\{\gamma, \gamma^{\vee}\right\}$, i.e. a framed curve defined via a choice of two curves $\gamma$ and $\gamma^{\vee}$ on the direct and dual lattices respectively, see Fig \ref{Fig:Framed_line}.
In the definition \eqref{eq:line_operators}, $p=0$ and $p=1$ correspond to the topological line operators in the toric code and double semion models respectively.
The commutators of these line operators have the form 
\begin{equation}
\begin{split}
    \mc W_{(\ms q_1, \ms m_1)}^{(p)}(L_1)
    \mc W_{(\ms q_2, \ms m_2)}^{(p)}(L_2) 
    &=   \left[S^{(p)}_{(\ms q_1, \ms m_1);(\ms q_2, \ms m_2)} \right]^{{\rm{Int}} (L_1,L_2)}  \mc W_{(\ms q_2, \ms m_2)}^{(p)}(L_2)  \mc W_{(\ms q_1, \ms m_1)}^{(p)}(L_1)\,.    
\end{split}
\end{equation}
Where $S^{(p)}_{(\ms q_1, \ms m_1);(\ms q_2, \ms m_2)}$ is the S-matrix element in the toric code and double semion theories for $p=0,1$ respectively, which is
\begin{equation}
S^{(p)}_{(\ms q_1, \ms m_1);(\ms q_2, \ms m_2)}=\exp\left\{i\pi \left(\ms q_1\ms m_2+\ms q_2\ms m_1 + p \ms m_1\ms m_2\right) \right\}\,.    
\end{equation}
\begin{figure}[h]
\begin{center}
\includegraphics[width=0.4\textwidth]{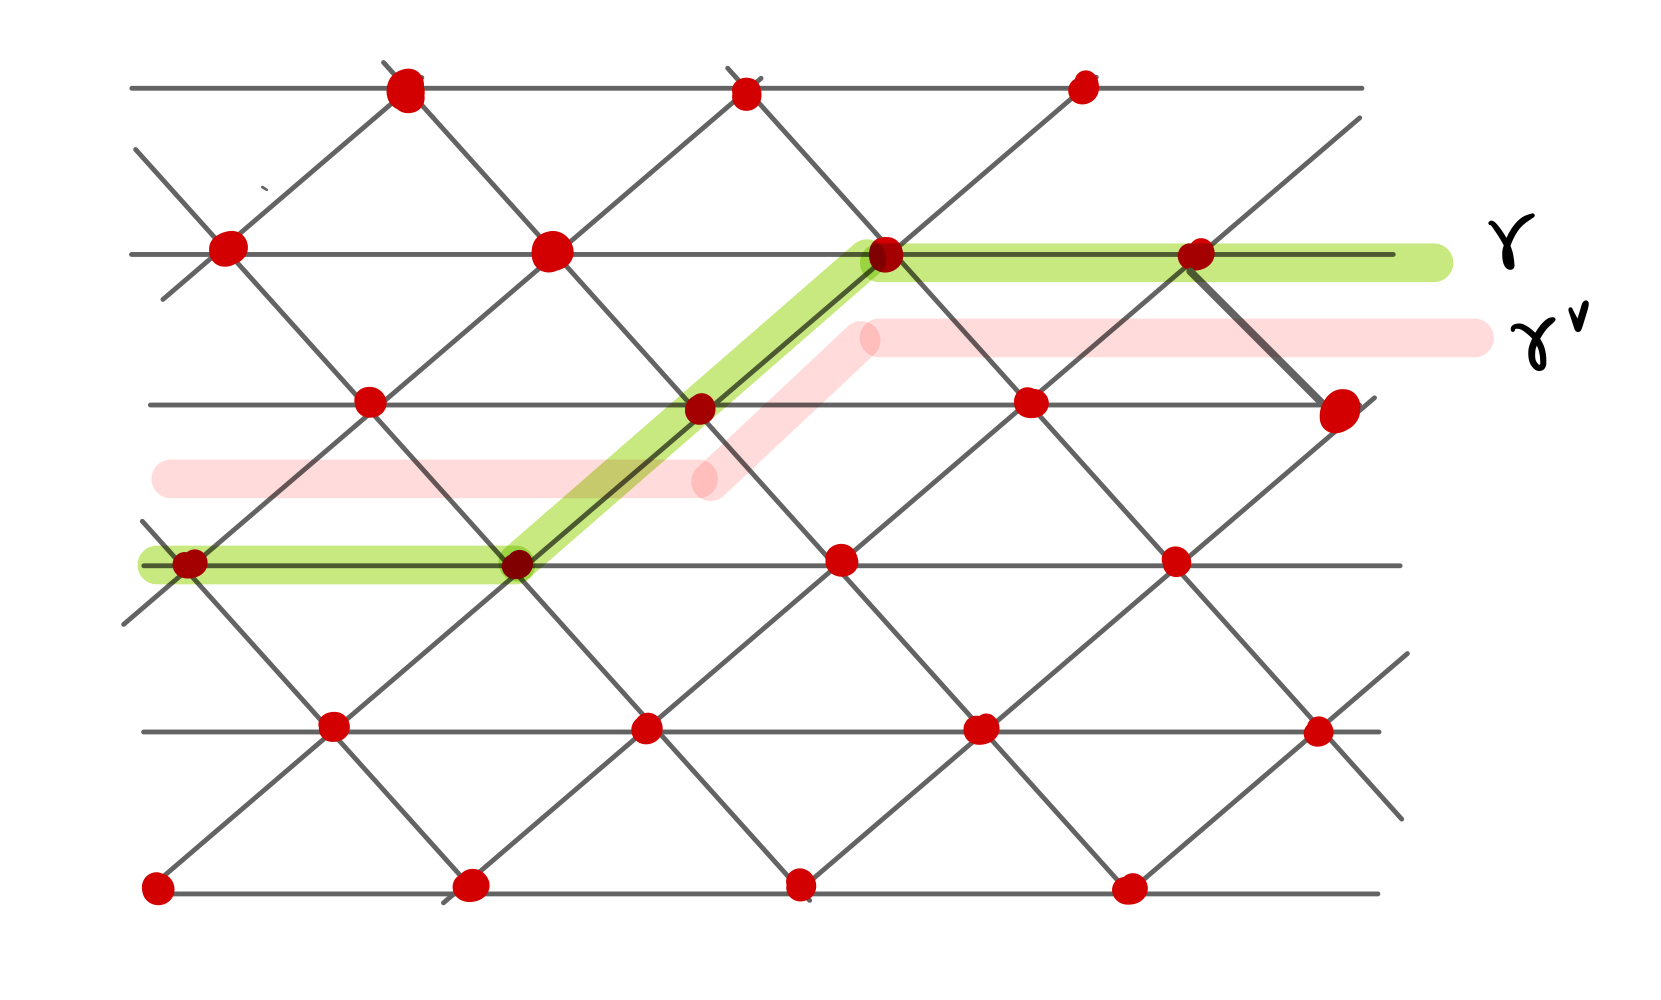}    
\end{center}
\caption{A general dyonic line requires a choice of framing, i.e., a choice of a curve $\gamma$ on the direct lattice and another nearby curve $\gamma^{\vee}$ on the dual lattice.}
\label{Fig:Framed_line}
\end{figure}
It immediately follows that all closed line operator mutually commute for both choices of $p$.
Since the Hamiltonians \eqref{eq:TC and DS in loop basis} are constructed from loop operators, this immediately implies the exact solvability of these models.

\newl The low energy subspace of the two models can be distinguished by the topological properties of the line operators that commute with these models.
In particular by the statistics of the `flux' line operators labelled as $(0,1)$. We find
\begin{equation}
\begin{split}
    \mc W_{(0, 1)}^{(p)}(L_1)
    \mc W_{(0,1)}^{(p)}(L_2) 
    &=   (-1)^{p{\rm{Int}} (L_1,L_2)}  \mc W_{(0,1)}^{(p)}(L_2)  \mc W_{(0,1)}^{(p)}(L_1)\,.    
\end{split}
\end{equation}
\AT{Maybe add something about the mixed anomaly for the emergent 1fs?}
