# Supplementary material for: Symmetry fractionalization, mixed-anomalies and dualities in quantum spin models with generalized symmetries
Source: arXiv:2307.01266 source file (2025-01-22)
Supplement: Supplementary file 3 [file generalizations_of_LevinGu.tex]

The $\mbb Z_2$ symmetric Levin-Gu SPT model \cite{Levin:2012yb} is defined on a triangular lattice with each vertex $\ms v$ endowed with a two dimensional on-site Hilbert space $\mc V_{\ms v}\cong \mbb C^2$. 
There is a natural action of the Pauli operators on the local Hilbert space. The fixed point Hamiltonian has the form
    \begin{equation}
        H_{\rm{LG}}=-\sum_{j}\sigma^x_j\prod_{\triangle_{jj_1j_
2}}\exp\left\{\frac{2 \pi i}{8}(1-\sigma_{j_1}^z\sigma_{j_2}^z)\right\}\,. 
    \end{equation}
    For the purposes of generalization toi $\mbb Z_n$ SPTs, it is convenient to slightly re-formulate the Levin-Gu model. Let us denote the hexagon comprising of the six triangles that contain the vertex $j$ as ${\rm{Hex}}_j$. Next we denote the edges of the lattice as $\ms e$ and denote the source and target of each oriented edge as $\ms{s(e)}$ and $\ms{t(e)}$ respectively. An operator $\mc O_{\ms e}$ can be defined on the edge $\ms e$ which essentially  maps the $\left\{+1,-1\right\}$ eigenvalues of $\sigma^{z}_{\ms{t(e)}}\sigma^{z}_{\ms{s(e)}}$ to $\left\{0,1\right\}$. Such an operator has the form 
    \begin{equation}
        \mc O_{\ms e}= \sum_{\mu\in 0,1}\mu \frac{1+\mu \sigma^{z}_{\ms{s(e)}}\sigma^{z}_{\ms{t(e)}}}{2}= \sum_{\mu\in 0,1}\mu P_{\ms e}^{(\mu)}\,.
    \end{equation}
    Using these operators, the Levin-Gu model can be rewritten as
    \begin{equation}
        \mc{H}_{\rm LG}=
        -\sum_{j}\sigma^{x}_{j}\exp\left\{\frac{2\pi i}{4}\sum_{\ms e\in \partial {\rm{Hex}_j}} \mc O_{\ms e}\right\}
        = -\sum_{j}\sigma^{x}_j\exp\left\{i\pi \oint_{\partial 
         {\rm{Hex}_j}
        }{\rm{Bock}}(A)\right\}\,,
    \end{equation}
where in the final expression, we have introduced a $\mbb Z_2$ gauge field whose configuration on a link $\ms e$ is the eigenvalue of $\sigma^{z}_{\ms{t(e)}}\sigma^{z}_{\ms{s(e)}}$.

\medskip \noindent With this preparation, the generalization to $\mbb Z_n$symmetric SPTs is straightforward. 
Let us consider an oriented triangulation of a manifold $\Sigma$, with each vertex $\ms v$ of the triangulation endowed with a Hilbert space $\mc V_{\ms v}\simeq \mbb C_n$.
There is an action of the $\mbb Z_n$ clock and shift algebra given by 
\begin{equation}
    Z^{(n)}_{\ms v}   X^{(n)}_{\ms v'}=e^{2\pi i \delta_{\ms v \ms v'}/n }    X^{(n)}_{\ms v'}\, Z^{(n)}_{\ms v} 
    \label{eq:Zn_clock_algebra}
\end{equation}
Let the global $\mbb Z_n$ symmetry be generated by $\mc U= \prod_{\ms v}X^{(n)}_{\ms v}$. There are a total of $n$ SPTs labelled by $p\in \mbb Z_n$ with the fixed point Hamiltonians
    \begin{equation}
    \begin{split}
        \mc{H}^{(\mbb Z_n,p)}&=
        -\sum_{\ms v}X^{(n)}_{\ms v}\exp\left\{\frac{2\pi ip}{n^2}\sum_{\ms e\in \partial {\rm{Hex}_j}} \mc O^{(n)}_{\ms e}\right\}+ \text{H.c} \\
        &= -\sum_{j}X^{(n)}_{\ms v}\exp\left\{\frac{2\pi ip}{n}\oint_{\partial 
         {\rm{Hex}_{\ms v}}
        }{\rm{Bock}}(A)\right\}+ \text{H.c}\,,     
        \label{eq:Zn_Levin_Gu_generalization}
    \end{split}
    \end{equation}
    where we have defined 
    \begin{equation}
        \begin{split}
            \mc O^{(n)}_{\ms e}&= \sum_{\mu\in \mbb Z_n} \mu P_{\ms e}^{(n,\mu)}\,, \\
            P_{\ms e}^{(n,\mu)}&= \frac{1}{n}\sum_{\tau=0}^{n-1}e^{-\frac{2\pi i\tau \mu}{n}}(Z^{(n)}_{\ms s(\ms e)}\left(Z^{(n)}_{\ms t(\ms e)})^{\dagger}\right)^{\tau}\,. 
        \end{split}
    \end{equation}
