# Supplementary material for: Symmetry fractionalization, mixed-anomalies and dualities in quantum spin models with generalized symmetries
Source: arXiv:2307.01266 source file (2025-01-22)
Supplement: Supplementary file 4 [file Calculation_duality_of_characters.tex]

In this appendix we detail the calculation of mapping of characters under gauging of $\mbb Z_2 \subset \mbb Z_4$, going from \eqref{eq:dual characters} to \eqref{eq:mapping of characters}. 
Firstly, inserting \eqref{eq:dual partition functions} into \eqref{eq:dual characters}, one gets
\begin{equation}
\begin{split}
    \chi_{\fr T^{\vee}}[q\,, \vec{\alpha}_{\ms n^{\vee}}\,,\alpha_{\ms k}\,,\ms n^{\vee}_t\,, \vec{\ms k}]&=\frac{1}{2^{2+N}}\sum_{\ms k_t,\vec{\ms n}^{\vee},\ms n_t.\vec{\ms n}}
    (-1)^{\alpha_{\ms k}\ms k_t+ \vec{\alpha}_{\ms n^{\vee}}\cdot \vec{\ms n}_{\vee}+ \ms n_{t}\ms n_{t}^{\vee}+ \vec{\ms n} \cdot\vec{\ms n}^{\vee} }\,.
\end{split}
\end{equation}
